# Supplementary material for: The 2D Ray Tracing Problem using ABCD Lenses and Mirrors is Turing Complete
Source: arXiv:2606.24218 source file (2026-06-23)
Supplement: Supplementary file 1 [file Appendix-A-TC.tex]

% !TEX root = ICALP_main.tex

\section{Appendix: Turing Completeness of Unitary Matrices Tiling}
\label{app:TC}

Here, we show how components of types 1 to 6 from Section~\ref{TC_system} can be used to simulate an RTM when no area constraints need to be considered. Afterwards, we show how a network of unitary matrices can be implemented using the presented tiling structure. Note that we use the terms \textbf{components} and \textbf{gadgets} synonymously throughout all our Appendices.

\subsection{Turing Completeness of Unitary Matrices Network}

For our simulation we will adapt the quadruple form of a RTM as discussed in~\cite{morita2017reversiblecomputing}. 

\begin{definition}[Reversible Turing Machine]
	A transition of the TM is either of the form
	\begin{itemize}
		\item a \textbf{computing transition}, i.e. a transition $[p, x, y, q]$ with states $p,q\in Q$ and symbols $x,y\in\Sigma$, or
		\item a \textbf{movement transition}, i.e. a transition $[p, \emptysymbol, d, q]$ with states $p,q\in Q$, a special symbol $\emptysymbol\not\in\Sigma$ (indicating that $x$ is not a symbol read from the tape) and a moving direction of the head $d\in\{-1,0,+1\}$.
	\end{itemize}
	We call the first form of a transition a \emph{computing transition} and the second a \emph{movement transition}.
	
	A DTM is a reversible DTM if for any pair of distinct quadruples
	$[p_1, x_1, y_1, q_1]$ and $[p_2, x_2, y_2, q_2]$ it holds that
	\begin{itemize}
		\item \textbf{Forward determinism:} if $p_1=p_2$ then $x_1\not=\emptysymbol$ and $x_2\not=\emptysymbol$ and $x_1\not=x_2$ and 
		\item \textbf{Backward determinism:} if $q_1=q_2$ then $x_1\not=\emptysymbol$ and $x_2\not=\emptysymbol$ and $y_1\not=y_2$.
	\end{itemize}
	In the following we assume that within a computation the RTM always alternates from step to step between computing and movement transition. 
	%
	%=====================
	%
	%A DTM is described by quadruples of the form [p, x, y, q], where: p is the source state, x is the symbol for read (or direction for move rules), y is the symbol for write (or direction for move rules) and q is the target state.
	%
	%A DTM is reversible if it is both forward deterministic and backward deterministic:
	%
	%\begin{itemize}
	%	\item \textbf{Forward determinism:} For any pair of distinct quadruples 
	%	$[p_1, x_1, y_1, q_1]$ and $[p_2, x_2, y_2, q_2]$, 
	%	if $p_1 = p_2$ then $x_1 \neq x_2$.
	%	\item \textbf{Backward determinism:} For any pair of distinct quadruples 
	%	$[p_1, x_1, y_1, q_1]$ and $[p_2, x_2, y_2, q_2]$, 
	%	if $q_1 = q_2$ then $y_1 \neq y_2$.
	%\end{itemize}
	%
	%
\end{definition}

To show how a unitary matrices network can simulate a RTM we have to solve two simulation tasks:
\begin{enumerate}
	\item simulating a \textbf{computing transition}, and 
	\item simulating a \textbf{movement transition}.
\end{enumerate}
Hence, based on our definition of a RTM the starting state of a transition can never be the starting state of computing transition as well as the stating state of an movement transition. This is based on the forward determinism of a RTM. Analogously, the resulting state of a transition can never be the resulting state of computing transition as well as the resulting state of an movement transition. This is based on the backward determinism of a RTM. 

We assume that each state is represented by a set of gadgets. A gadget is active, if this is indicated by the token arriving at the gadget via an incoming edge $\particle_{\text{in}}$ having at least one feature $\feature_{\text{in}, 1}$ or $\feature_{\text{in}, 2}$ with a value different from 0. We assume that the value of $\feature_{\text{in}, 1}$ represents the tape content of the RTM to the right of the current head position (including the current cell) and the value of $\feature_{\text{in}, 2}$ represents the tape content of the RTM to the left of the current head position.

\subsubsection{Simulating a Computing Transition}

The collection of gadgets which represent a state are
\begin{itemize}
	\item one gadget $G_S$ for splitting,
	\item may be one gadget for shifting down $G_{R,1}$ by a base value $b=1$, and
	\item may be one gadget for shifting up $G_{A,0}$ by a base value $b=1$. 
\end{itemize}
Let us focus on the simulation of the transitions from a state $p$, i.e. the two transitions $[p,0,y_0,q_0]$ and $[p,1,y_1,q_1]$. Assume that the RTM is in state $p$ and therefore the gadget $G_S$ is active. To determine the correct symbol of the cell of the head we assume that for the next transition $[p,x,y,q]$
$$
x \ \ = \ \ \left\{\begin{array}[c]{ll}
0 & \text{if } \feature_{\text{in}, 1} < 1\\
1 & \text{if } \feature_{\text{in}, 1} > 1\ .
\end{array}\right.
$$ 
Recall that we assume that the values 0, 1, and 2 never occur. According to the splitting of $G_S$ we assume that the first output $\particle_{\text{out}, 1}$ represents $x=0$ and the second output $\particle_{\text{out}, 2}$ represents $x=1$.
Recall that only one of the output edges will get the token. Based on $x$ we distinguish between the following cases:
\begin{enumerate}
	\item $x=0$ and hence $\particle_{\text{out}, 1}$ will activate its connected successor gadget. We distinguish between two possible transitions (only one will be defined as a transition of the RTM):
	\begin{itemize}
		\item $[p,0,0,q_0]$ then the state $p$ final output edge will be $\particle_{\text{out}, p, 0}=\particle_{\text{out}, 1}$ or
		\item $[p,0,1,q_0]$ then we connect $\particle_{\text{out}, 1}$ with the input $\particle_{\text{in}}'$ of the shifting up gadget $G_{A,0}$ and its output object will be the final output edge $\particle_{\text{out}, p, 1}=\particle_{\text{out}}'$ of system simulating the state $p$.
	\end{itemize}
	\item $x=1$ and hence $\particle_{\text{out}, 2}$ will activate its connected gadget. We distinguish between two possible transitions (only one will be successor defined as a transition of the RTM):
	\begin{itemize}
	\item $[p,1,0,q_1]$ then we connect $\particle_{\text{out}, 2}$ with the input $\particle_{\text{in}}'$ of shifting down gadget $G_{R,1}$ and its output edge will be the final output edge $\particle_{\text{out}, p, 0}=\particle_{\text{out}}'$ of the state $p$ or
	\item $[p,1,1,q_1]$ then the state $p$ final output edge will be $\particle_{\text{out}, p, 1}=\particle_{\text{out}, 2}$.
	\end{itemize}
\end{enumerate}

\subsubsection{Simulating a Movement Transition}

Recall that we have assumed that computing and movement transitions will alternate. Hence we can implement the joining of a splitting of the simulation of the computing transition at the beginning of the simulation of the movement transition.

Based on the backward determinism we know that there are at most 2 different transitions $[p',x,y,p]$ and $[p'',x',y',p]$ having the same next state $p$. Moreover we know that for these transitions the currently written symbol into a cell is different. Hence, the two available output edges $\particle_{\text{out}, p', y}$
and $\particle_{\text{out}, p'', y'}$ of the predecessor states of $p$ are uniquely defined. W.l.o.g. assume that these are $\particle_{\text{out}, p', 0}$ and $\particle_{\text{out}, p'', 1}$.

Hence we can start the simulation of a movement transition by a joining gadget where 
we assume that $\particle_{\text{in}, 1}$ will be used for the feature value $\feature_1<1$ and $\particle_{\text{in}, 2}$ will be used for the feature value $\feature_1>1$. In this case we connect $\particle_{\text{out}, p', 0}$ with $\particle_{\text{in}, 1}$ and $\particle_{\text{out}, p'', 1}$ with $\particle_{\text{in}, 2}$. The output edge $\particle_{\text{out}, J}$ of the 
joining gadget $G_J$ will denote the main starting edge $\particle_{\text{in}, m}$ of the movement transition simulation. Let $\particle_{\text{out}, m}$ denote the output edge of the movement simulation.

For a movement transition we distinguish between the following transitions:
\begin{enumerate}
	\item $[p,\emptysymbol,0,q]$: In the case \emph{do not move} we identify $\particle_{\text{out}, m}=\particle_{\text{in}, m}$.
	\item $[p,\emptysymbol,+1,q]$: In the case \emph{move to the right} we proceed as follows.
	\begin{enumerate}
		\item We start by using a splitting gadget $G_S$ where its input edge  $\particle_{\text{in}, S}$ is given by $\particle_{\text{in}, m}$. We assume that its first output edge $\particle_{\text{out}, S, 1}$ is used for the token if the first feature is smaller than 1, and its second output edge $\particle_{\text{out}, S, 2}$ is used for the token if the first feature is larger than 1.
		\item We connect the second output edge $\particle_{\text{out}, S, 2}$ with a shifting down gadget $G_R$ with output edge $\particle_{\text{out}, R, 1}$.
		\item We connect each of the unconnected output edges $\particle_{\text{out}, S, 1}$ and $\particle_{\text{out}, R, 1}$ with the input edges of a multiplying gadget $G_{M,1}$ and $G_{M,2}$, i.e. $\particle_{\text{out}, S, 1}$ with $\particle_{\text{in}, M, 1}$ and
		$\particle_{\text{out}, R, 1}$ with $\particle_{\text{in}, M, 2}$. Let 
		$\particle_{\text{out}, M, 1}$ and $\particle_{\text{out}, M, 2}$ be the corresponding output edges.
		\item We connect each of the output edges to an input edge of a switching gadget (let $G_{C,1}$ and $G_{C,1}$ be the two gadgets), let 
		$\particle_{\text{out}, C, 1}$ and $\particle_{\text{out}, C, 2}$ be the corresponding output edges.
		\item We connect the second output edge $\particle_{\text{out}, C, 2}$ with a shifting up gadget $G_A$ with output edge $\particle_{\text{out}, A, 1}$.
		\item Using a joining gadget $G_J$ where $\particle_{\text{in}, J, 1}$ is connected with $\particle_{\text{out}, C, 1}$ and $\particle_{\text{in}, J, 2}$ is connected with $\particle_{\text{out}, A, 1}$. Let $\particle_{\text{out}, J}$ be the resulting output edge. Note that for the values of first feature of the token at the input edges $\particle_{\text{in}, J, 1}$ and $\particle_{\text{in}, J, 2}$ we can see that the first feature of a token at $\particle_{\text{in}, J, 1}$ is smaller than 1, where the first feature of token at $\particle_{\text{in}, J, 2}$ is larger than 1.
		\item Finally we perform a sequence of three three switching gadgets (we need a sequence of three to avoid negative values in Step d above). The output edge of the last switching gadget will be the resulting output edge $\particle_{\text{out}, m}$.
	\end{enumerate}
	\item $[p,\emptysymbol,-1,q]$: In the case \emph{move to the left} we proceed as follows.
	\begin{enumerate}
		\item We start by using a switching gadget $G_{C}$ which input $\particle_{\text{in}, C}$ is given by $\particle_{\text{in}, m}$.
		Let $\particle_{\text{out}, C}$ be the corresponding output edge.
		\item We continue by using a splitting gadget $G_S$ where its input edge  $\particle_{\text{in}, S}$ is given by $\particle_{\text{out}, C}$. We assume that its first output edge $\particle_{\text{out}, S, 1}$ will get the token if the first feature of the token is smaller than 1, and its second output edge $\particle_{\text{out}, S, 2}$ will get the token if the first feature of the token is larger than 1.
		\item We connect the second output edge $\particle_{\text{out}, S, 2}$ with a shifting down gadget $G_R$ with output edge $\particle_{\text{out}, R, 1}$.
		\item We connect each of the unconnected output edges $\particle_{\text{out}, S, 1}$ and $\particle_{\text{out}, R, 1}$ with the input edges of a multiplying gadget $G_{M,1}$ and $G_{M,2}$, i.e. $\particle_{\text{out}, S, 1}$ with $\particle_{\text{in}, M, 1}$ and
		$\particle_{\text{out}, R, 1}$ with $\particle_{\text{in}, M, 2}$. Let 
		$\particle_{\text{out}, M, 1}$ and $\particle_{\text{out}, M, 2}$ be the corresponding output edges of the multiplying gadgets.
		\item Next we perform at each of the output edges 
		a sequence of three three switching gadgets (we need a sequence of three to avoid negative values in Step d above). 
		Let $\particle_{\text{out}, C,1}$ and $\particle_{\text{out}, C,2}$ be the 
		output edges of the two last switching gadgets. Note that based on the multiplication gadgets the first feature of a token at both output edges is smaller than 1.
		\item We connect $\particle_{\text{out}, C,2}$ with an shifting up gadget with output edge $\particle_{\text{out}, A}$. Note that the first feature of 
		an token at $\particle_{\text{out}, C,1}$ is smaller than 1 and the first feature of a token at 
		$\particle_{\text{out}, A}$ is larger than 1.
		\item Finally we use a joining gadgets $G_J$ where $\particle_{\text{in}, J, 1}$ is connected with $\particle_{\text{out}, C, 1}$ and $\particle_{\text{in}, J, 2}$ is connected with $\particle_{\text{out}, A}$. Let $\particle_{\text{out}, J}$ be the resulting output edge. The output edge of the joining gadget will be the resulting final output edge $\particle_{\text{out}, m}$.
	\end{enumerate}
\end{enumerate}
Based on the construction above one can see that the sequence of activated gadgets represents the sequence of reached states within the computation of a RTM, and the sequence of feature values $\feature_1$ and $\feature_2$ of the activated gadgets represents the sequence of configurations of the computation of a RTM. Hence the sequences simulate a RTM and therefore we can conclude:\\

\noindent
{\bf Theorem~\ref{th:UMNP}.} \emph{Unitary matrices network problem built by gadgets of type 1 to 6 is Turing complete, if no explicit connecting gadget from the output of one gadget to the input of other gadgets is required.}

\subsection{Turing Completeness of Unitary Matrices Tiling}

To simulate a RTM by the unitary matrices tiling problem we use the simulation of the unitary matrices network problem and analyse how the used gadgets can be located in the plane. Figure~\ref{fig:LensTileTypes_001} illustrates the types of gadgets.

\begin{figure}[htb]
	\begin{center}
			\scalebox{.50}{
					\input{fig/LensTileTypes_002.pspdftex}
				}
		\end{center}
	\caption{
			Illustration of the tiles of the different types of gadgets.
			\label{fig:LensTileTypes_001}}
\end{figure}

Using these building blocks we can implement the simulation of the computation transition as presented in Figure~\ref{fig:LensTileTypes_p00q_001} for $[p,0,0,q_0]$, Figure~\ref{fig:LensTileTypes_p01q_001} for $[p,0,1,q_0]$, Figure~\ref{fig:LensTileTypes_p10q_001} for $[p,1,0,q_1]$, and Figure~\ref{fig:LensTileTypes_p11q_001} for $[p,1,1,q_1]$.
The constructions for the simulation of the movement transition are presented in Figure~\ref{fig:LensTileTypes_p_0q_001} for $[p,\emptysymbol,0,q]$, Figure~\ref{fig:LensTileTypes_p_+q_002} for $[p,\emptysymbol,+1,q]$, and Figure~\ref{fig:LensTileTypes_p_-q_002} for $[p,\emptysymbol,-1,q_1]$. As one can see, some distance gadgets have to be added to extent the alternative ways of the active gadgets. One can easily verify that the construction presented in Figure~\ref{fig:LensTileTypes_p00q_001} to~\ref{fig:LensTileTypes_p_-q_002} can be connected via distance and crossing gadgets to generate from an RTM a unitary matrices tiling instance. If the input is encoded by the binary representation of the value of first feature $\feature_1$ of the input object of the construction representing the starting state of the RTM we can conclude the claim of Theorem~\ref{th:UMTP}.\\

\noindent
{\bf Theorem~\ref{th:UMTP}.} \emph{Unitary matrices tiling problem is Turing complete.}

\begin{figure}[htb]
	\begin{center}
		\scalebox{.50}{
			\input{fig/LensTileTypes_p00q_001.pspdftex}
		}
	\end{center}
	\caption{
		Illustration of the implementation of the transition $[p,0,0,q_0]$.
		\label{fig:LensTileTypes_p00q_001}}
\end{figure}

\begin{figure}[htb]
	\begin{center}
		\scalebox{.50}{
			\input{fig/LensTileTypes_p01q_002.pspdftex}
		}
	\end{center}
	\caption{
		Illustration of the implementation of the transition $[p,0,1,q_0]$.
		\label{fig:LensTileTypes_p01q_001}}
\end{figure}

\begin{figure}[htb]
	\begin{center}
		\scalebox{.50}{
			\input{fig/LensTileTypes_p10q_002.pspdftex}
		}
	\end{center}
	\caption{
		Illustration of the implementation of the transition $[p,1,0,q_1]$.
		\label{fig:LensTileTypes_p10q_001}}
\end{figure}

\begin{figure}[htb]
	\begin{center}
		\scalebox{.50}{
			\input{fig/LensTileTypes_p11q_001.pspdftex}
		}
	\end{center}
	\caption{
		Illustration of the implementation of the transition $[p,1,1,q_1]$.
		\label{fig:LensTileTypes_p11q_001}}
\end{figure}

\begin{figure}[htb]
	\begin{center}
		\scalebox{.50}{
			\input{fig/LensTileTypes_p_0q_001.pspdftex}
		}
	\end{center}
	\caption{
		Illustration of the implementation of the movement transition $[p,\emptysymbol,0,q]$.
		\label{fig:LensTileTypes_p_0q_001}}
\end{figure}

\begin{figure}[htb]
	\begin{center}
		\scalebox{.50}{
			\input{fig/LensTileTypes_p_pq_003.pspdftex}
		}
	\end{center}
	\caption{
		Illustration of the implementation of the movement transition $[p,\emptysymbol,+1,q]$.
		\label{fig:LensTileTypes_p_+q_002}}
\end{figure}

\begin{figure}[htb]
	\begin{center}
		\scalebox{.50}{
			\input{fig/LensTileTypes_p_mq_003.pspdftex}
		}
	\end{center}
	\caption{
		Illustration of the implementation of the movement transition $[p,\emptysymbol,-1,q]$.
		\label{fig:LensTileTypes_p_-q_002}}
\end{figure}

\clearpage

\newpage
