# Supplementary material for: The 2D Ray Tracing Problem using ABCD Lenses and Mirrors is Turing Complete
Source: arXiv:2606.24218 source file (2026-06-23)
Supplement: Supplementary file 2 [file Appendix-C-LensSystem.tex]

% !TEX root = ICALP_main.tex

\section{Construction of Optical Lens Gadgets}
\label{app:ConstOLG}

Within the construction of optical lens gadgets we have used often diagonal mirrors.

\begin{figure}[htb]
	\begin{center}
		\scalebox{.30}{
			\input{fig/LensScapes_ThinLens_05.pspdftex}
		}
	\end{center}
	\caption{
		An optical system given by two plain mirrors.
		\label{fig:AppThinLens_05}}
\end{figure}

If a ray is reflected on two diagonal mirrors we can conclude from Figure~\ref{fig:AppThinLens_05}:

\begin{observation}
	Assume that a ray particle is reflected off two parallel diagonal mirrors, then the angle of the ray relative to the x-axis after the second reflection equals the original angle. If the two mirrors are orthogonal to each other, then the angle after the reflection will be $\pi-\theta$, if $\theta$ is the original angle. 
\end{observation}

Using the construction of $M_\text{wire}$ combined with diagonal mirrors we can construct a network of wires in 2D connecting different gadgets which will help us to simulate an RTM. Each gadget will have some kind of its own (virtual) x-axis for determining the height of the incoming and outgoing ray particles. Analogously, we can also turn the gadgets, such that the y-axis will take over the role of the x-axis in our previous construction (i.e. the angle and the distance might be measured relative to the y-axis). If the maximum distance and the maximum angle
% used in our constructions 
are small enough we can place the mirrors within the first optical system $S_{d_0}$ within our constructions above and with the effect that no mirror or lens stands in the way of some other constructed gadgets, e.g. we can include a mirror system like presented in Figure~\ref{fig:AppThinLens_05} inside of the optical system $S_{d_0}$.

Using such a setting we can implement a vertical shift of the ray particle's potential paths by a construction as given in Figure~\ref{fig:AppThinLens_07}. Building a connection between some optical systems which simulates some aspects of the RTM computation, one can use a combination of some 
construction for $M_\text{wire}$ with some diagonal mirrors as illustrated in Figure~\ref{fig:AppThinLens_09}. Recall that to guarantee that the in-going angle equals the out-going, we have to ensure that, after traveling through the contraction, the ray goes in the same direction as before. Furthermore, we have to guarantee that the length of the path which the ray travels between any pair of lenses does not depend on the starting height of the ray.

\begin{figure}[htb]
	\begin{center}
		\scalebox{.30}{
			\input{fig/LensScapes_ThinLens_07.pspdftex}
		}
	\end{center}
	\caption{
		An optical system for shifting the potential ray particle ways.
		\label{fig:AppThinLens_07}}
\end{figure}

\begin{figure}[htb]
	\begin{center}
		\scalebox{.30}{
			\input{fig/LensScapes_ThinLens_09.pspdftex}
		}
	\end{center}
	\caption{
		An optical system for connecting an optical system located at {\bf in} with an optical system located at {\bf out}. 
		\label{fig:AppThinLens_09}}
\end{figure}

For splitting based on the middle of the height offset we can use a construction as illustrated in Figure~\ref{fig:AppThinLens_08}.

\begin{figure}[htb]
	\begin{center}
		\scalebox{.30}{
			\input{fig/LensScapes_ThinLens_08.pspdftex}
		}
	\end{center}
	\caption{
		An optical system for splitting the height offset in the middle.
		\label{fig:AppThinLens_08}}
\end{figure}

The correctness of the construction in Figure~\ref{fig:AppThinLens_08} follows from the observation that, if we assume the following scenarios:
\begin{itemize}
	\item assume an optical system where the ray travel through space
	\item assume that the rays might reach the end of the system at a virtual vertical line of length $\ell$. Let us denote the lower end of this line by a base point $b$
	\item assume that a ray particle $r$ reaches the end line at height $h\le \ell$ with an angle of $\theta$ (relative to a horizontal line).
\end{itemize} 
Now we insert a diagonal mirror into this optical system going through the base point $b$. Let us investigate the ray particle $r$. We have
\begin{enumerate}
	\item $r$ passes the virtual horizontal end line going through the base point $b$ by traveling the same distance as it would without the diagonal mirror when passing the virtual vertical end line
	\item $r$ passes the virtual horizontal end line going through the base point $b$ at a distance of $\ell$ from $b$
	\item $r$ will have an angle of $\theta$ (relative to a vertical line) and passes the virtual horizontal end line going through the base point $b$.
\end{enumerate}
Figure~\ref{fig:AppThinLens_08a} and~\ref{fig:AppThinLens_08b} illustrate the two different paths of the lower and upper halves of the height offset.

%\begin{figure}[htb]
%	\begin{center}
	%		\scalebox{.30}{
		%			\input{fig/LensScapes_ThinLens_08a.pspdftex}
		%		}
	%	\end{center}
%	\caption{
	%		An optical system for splitting the height offset in the middle. The way of the lower half of the height offset is highlighted. 
	%		\label{fig:AppThinLens_08a}}
%\end{figure}
%
%
%\begin{figure}[htb]
%	\begin{center}
	%		\scalebox{.30}{
		%			\input{fig/LensScapes_ThinLens_08b.pspdftex}
		%		}
	%	\end{center}
%	\caption{
	%	An optical system for splitting the height offset in the middle. The way of the upper half of the height offset is highlighted. 
	%		\label{fig:AppThinLens_08b}}
%\end{figure}

\begin{figure}[htb]
	\centering
	\begin{minipage}[t]{0.35\textwidth}
		\centerline{
			\scalebox{.18}{
				\input{fig/LensScapes_ThinLens_08a.pspdftex}
		}}
		
		\caption{
			An optical system for splitting the height offset in the middle. The way of the lower half of the height offset is highlighted. 
			\label{fig:AppThinLens_08a}}
		%\end{figure}
	\end{minipage} 
	\hspace*{0.1\textwidth}
	\begin{minipage}[t]{0.35\textwidth}
		%\begin{figure}[H]
		\centerline{
			\scalebox{.18}{
				\input{fig/LensScapes_ThinLens_08b.pspdftex}
		}}
		\caption{
			An optical system for splitting the height offset in the middle. The way of the upper half of the height offset is highlighted. 
			\label{fig:AppThinLens_08b}}
	\end{minipage} 
	
\end{figure}

%A similar construction as in Figure~\ref{fig:AppThinLens_08} can be used for joining two possible ways. For this we have to guarantee that the ray from the upper paths starts with a height within the upper halve of the potential ways, and the from the lower paths starts with a height within the lower halve of the potential ways (see Figure~\ref{fig:AppThinLens_10}).
A similar construction as in Figure~\ref{fig:AppThinLens_08} can be used for joining two possible paths. For this we have to guarantee that the ray from the upper part starts with a height within the upper half of the potential paths, and then from the lower part, it starts with a height within the lower half of the potential paths (see Figure~\ref{fig:AppThinLens_10}).

\begin{figure}[htb]
	\begin{center}
		\scalebox{.30}{
			\input{fig/LensScapes_ThinLens_10.pspdftex}
		}
	\end{center}
	\caption{
		An optical system for joining non overlapping height offsets.
		\label{fig:AppThinLens_10}}
\end{figure}

To add or subtract $1$ from the height offset (to implement a shifting up and shifting down gadget) we can use a construction as illustrated in Figure~\ref{fig:AppThinLens_11}. Note that both constructions solve this task by shifting the horizontal baseline of the optical systems. To prohibit this one can use the constructions illustrated in Figure~\ref{fig:AppThinLens_12} and~\ref{fig:AppThinLens_13}.

\begin{figure}[htb]
	\begin{center}
		\scalebox{.30}{
			\input{fig/LensScapes_ThinLens_11.pspdftex}
		}
	\end{center}
	\caption{
		Promising that the height offset is not in the interval $[0,1)$ (i.e. the height offset is in the interval $[1, 2]$) the construction in a) subtracts $1$ from the height offset (shifting down). And promising that the height offset is not in the interval $(1, 2]$ (i.e. the height offset is in the interval $[0,1)$) the construction in b) adds $1$ to the height offset (shifting up).
		\label{fig:AppThinLens_11}}
\end{figure}

\begin{figure}[htb]
	\begin{center}
		\scalebox{.30}{
			\input{fig/LensScapes_ThinLens_12.pspdftex}
		}
	\end{center}
	\caption{
		Promising that the height offset is not in the interval $(1, 2]$ (i.e. the height offset is in the interval $[0,1)$) the construction adds $1$ to the height offset without changing the baseline, i.e. the baseline of the optical system on the input equals the baseline of the output (see green dashed line). This gives us an implementation of the shifting up gadget.
		\label{fig:AppThinLens_12}}
\end{figure}

\begin{figure}[htb]
	\begin{center}
		\scalebox{.30}{
			\input{fig/LensScapes_ThinLens_13.pspdftex}
		}
	\end{center}
	\caption{
		Promising that the height offset is not in the interval $[0,1)$ (i.e. the height offset is in the interval $[1, 2]$) the construction subtracts $1$ from the height offset without changing the baseline, i.e. the baseline of the optical system on the input equals the baseline of the output (see green dashed line). This gives us an implementation of the shifting down gadget.
		\label{fig:AppThinLens_13}}
\end{figure}

\clearpage

\newpage
